# Supplementary material for: Online, Informative MCMC Thinning with Kernelized Stein Discrepancy
Source: arXiv:2201.07130 source file (2022-04-21)
Supplement: Supplementary file 1 [file supplement.tex]

%%%%%%%% ICML 2021 EXAMPLE LATEX SUBMISSION FILE %%%%%%%%%%%%%%%%%

\documentclass{article}
\usepackage{xr}
\makeatletter
\newcommand*{\addFileDependency}[1]{% argument=file name and extension
  \typeout{(#1)}
  \@addtofilelist{#1}
  \IfFileExists{#1}{}{\typeout{No file #1.}}
}
\makeatother

\newcommand*{\myexternaldocument}[1]{%
    \externalcitedocument{#1}%
    \addFileDependency{#1.tex}%
    \addFileDependency{#1.aux}%
}
\myexternaldocument{main}
% Recommended, but optional, packages for figures and better typesetting:
\usepackage{microtype}
\usepackage{graphicx}
\usepackage{subfigure}
\usepackage{booktabs} % for professional tables

% hyperref makes hyperlinks in the resulting PDF.
% If your build breaks (sometimes temporarily if a hyperlink spans a page)
% please comment out the following usepackage line and replace
% \usepackage{icml2021} with \usepackage[nohyperref]{icml2021} above.
\usepackage{hyperref}

% Attempt to make hyperref and algorithmic work together better:
%\newcommand{\theHalgorithm}{\arabic{algorithm}}

% Use the following line for the initial blind version submitted for review:
\usepackage{icml2021}

% If accepted, instead use the following line for the camera-ready submission:
%\usepackage[accepted]{icml2021}

% The \icmltitle you define below is probably too long as a header.
% Therefore, a short form for the running title is supplied here:
\icmltitlerunning{Online KSD Pruning}

\usepackage[ruled,vlined]{algorithm2e}
\usepackage{algorithmic}
\usepackage{amsmath}
\usepackage{amsmath}

\usepackage{amsopn}
\usepackage{amssymb}
\usepackage{xcolor}
% \DeclareMathOperator{\diag}{diag}
% \newtheorem{lemma}{Lemma}
% \newtheorem{theorem}{Theorem}
% \newtheorem{corollary}{Corollary}
% \newtheorem{definition}{Definition}
% \newcommand{\ten}[1]{\mathbfcal{#1}} %mathcal
% \newcommand{\mat}[1]{\mathbf{#1}}
% \newcommand{\ch}[1]{\textcolor{purple}{CH: #1}}
% \newcommand{\ak}[1]{\textcolor{blue}{AK: #1}}
% \newcommand{\dict}{\mat{D}}
% \newcommand{\seq}{\mat{S}}
% %\newcommand{\ksd}{D_{\mathcal{K}_0,p}}
% %\newcommand{\ksd}{\text{KSD}}
% \usepackage{pifont}
% \newcommand{\cmark}{\ding{51}}%
% \newcommand{\xmark}{\ding{55}}%
% \newcommand{\ksd}{{\rm KSD}}
% \begin{document}
% \appendix

% \onecolumn
% \input{sections/convergence_appendix}
% \newpage
% \input{sections/experiments_appendix}
% \newpage
% \input{sections/misc_appendix}

% \bibliography{references}
% \bibliographystyle{icml2021}
% \end{document}
